# Supplementary material for: Local Noncollinear Spin Analysis
Source: arXiv:1711.00919 source file (2017-11-02)
Supplement: Supplementary file 1 [file Local_Spin_Supplementary.pdf]

# Supporting information for:

# Local Noncollinear Spin Analysis

Bayileyegn A. Abate, Rajendra P. Joshi, and Juan E. Peralta*

*Department of Physics and Science of Advanced Materials, Central Michigan University, Mount Pleasant, MI, 48859, USA*

E-mail: peral1j@cmich.edu

*To whom correspondence should be addressed

## Derivation of Eq. 10 and Eq. 11 from the main text

Starting form Eq. 8 from the main text,

$$\begin{aligned}\langle \hat{\mathbf{S}}_A \cdot \hat{\mathbf{S}}_B \rangle &= \frac{3}{4}\delta_{AB}\sum_m \langle m \,|\, \hat{P}_A \,|\, m \rangle + \\ &\frac{1}{2}\sum_{m,n}\Big[ \langle mn \,|\, \hat{\mathbf{S}}_1 \cdot \hat{\mathbf{S}}_2 [\hat{P}_A\hat{P}_B + \hat{P}_B\hat{P}_A] \,|\, mn \rangle - \\ &\langle mn \,|\, \hat{\mathbf{S}}_1 \cdot \hat{\mathbf{S}}_2 [\hat{P}_A\hat{P}_B + \hat{P}_B\hat{P}_A] \,|\, nm \rangle \Big], \end{aligned} \tag{1}$$

where $m$ and $n$ label two-component spinors, which can be expressed as $|m\rangle = |m^{\uparrow}\rangle + |m^{\downarrow}\rangle$ and $|n\rangle = |n^{\uparrow}\rangle + |n^{\downarrow}\rangle$. Using this, we rewrite Eq. 1 as,

$$\begin{aligned}&\langle \hat{\mathbf{S}}_A \cdot \hat{\mathbf{S}}_B \rangle = \frac{3}{4}\delta_{AB}\Big[\sum_m \langle m^{\uparrow} \,|\, \hat{P}_A \,|\, m^{\uparrow} \rangle + \sum_m \langle m^{\downarrow} \,|\, \hat{P}_A \,|\, m^{\downarrow} \rangle\Big] \\ &+\frac{1}{2}\sum_{m,n}\Big[ \langle m^{\uparrow}n^{\uparrow} \,|\, \hat{\mathbf{S}}_1 \cdot \hat{\mathbf{S}}_2 [\hat{P}_A\hat{P}_B + \hat{P}_B\hat{P}_A] \,|\, m^{\uparrow}n^{\uparrow} \rangle - \langle m^{\uparrow}n^{\uparrow} \,|\, \hat{\mathbf{S}}_1 \cdot \hat{\mathbf{S}}_2 [\hat{P}_A\hat{P}_B + \hat{P}_B\hat{P}_A] \,|\, n^{\uparrow}m^{\uparrow} \rangle \Big] \\ &+\frac{1}{2}\sum_{m,n}\Big[ \langle m^{\downarrow}n^{\downarrow} \,|\, \hat{\mathbf{S}}_1 \cdot \hat{\mathbf{S}}_2 [\hat{P}_A\hat{P}_B + \hat{P}_B\hat{P}_A] \,|\, m^{\downarrow}n^{\downarrow} \rangle - \langle m^{\downarrow}n^{\downarrow} \,|\, \hat{\mathbf{S}}_1 \cdot \hat{\mathbf{S}}_2 [\hat{P}_A\hat{P}_B + \hat{P}_B\hat{P}_A] \,|\, n^{\downarrow}m^{\downarrow} \rangle \Big] \\ &+\frac{1}{2}\sum_{m,n}\Big[ \langle m^{\uparrow}n^{\downarrow} \,|\, \hat{\mathbf{S}}_1 \cdot \hat{\mathbf{S}}_2 [\hat{P}_A\hat{P}_B + \hat{P}_B\hat{P}_A] \,|\, m^{\uparrow}n^{\downarrow} \rangle - \langle m^{\uparrow}n^{\downarrow} \,|\, \hat{\mathbf{S}}_1 \cdot \hat{\mathbf{S}}_2 [\hat{P}_A\hat{P}_B + \hat{P}_B\hat{P}_A] \,|\, n^{\downarrow}m^{\uparrow} \rangle \Big] \\ &+\frac{1}{2}\sum_{m,n}\Big[ \langle m^{\downarrow}n^{\uparrow} \,|\, \hat{\mathbf{S}}_1 \cdot \hat{\mathbf{S}}_2 [\hat{P}_A\hat{P}_B + \hat{P}_B\hat{P}_A] \,|\, m^{\downarrow}n^{\uparrow} \rangle - \langle m^{\downarrow}n^{\uparrow} \,|\, \hat{\mathbf{S}}_1 \cdot \hat{\mathbf{S}}_2 [\hat{P}_A\hat{P}_B + \hat{P}_B\hat{P}_A] \,|\, n^{\uparrow}m^{\downarrow} \rangle \Big]. \end{aligned} \tag{2}$$

It is convenient at this point to label the terms containing $\hat{\mathbf{S}}_1 \cdot \hat{\mathbf{S}}_2$ from $A$-$H$:

$$\langle \hat{\mathbf{S}}_A \cdot \hat{\mathbf{S}}_B \rangle = \frac{3}{4}\,\delta_{AB}\,X + \frac{1}{2}[(A-B)+(C-D)+(E-F)+(G-H)]. \tag{3}$$

Now, we evaluate each of these terms separately. To this end, we make use of the following relations:

$$
\begin{aligned}
\hat{\mathbf{S}}_1 \cdot \hat{\mathbf{S}}_2 = \hat{S}_z(1)\hat{S}_z(2) + \frac{1}{2}[\hat{S}^+(1)\hat{S}^-(2) + \hat{S}^-(1)\hat{S}^+(2)], \\
\hat{S}_z(1)\,|m^{\uparrow}\rangle = \frac{1}{2}\,|m^{\uparrow}\rangle\,, \\
\hat{S}_z(1)\,|m^{\downarrow}\rangle = -\frac{1}{2}\,|m^{\downarrow}\rangle\,, \\
\hat{S}^+(1)\,|m^{\uparrow}\rangle = 0, \\
\hat{S}^-(1)\,|m^{\downarrow}\rangle = 0, \\
\hat{S}^-(1)\,|m^{\uparrow}\rangle = |m^{\downarrow}\rangle\,, \quad \text{and} \\
\hat{S}^+(1)\,|m^{\downarrow}\rangle = |m^{\uparrow}\rangle\,.
\end{aligned} \tag{4}
$$

The first term is

$$
A = \sum_{m,n} \left\langle m^{\uparrow} n^{\uparrow} \right| \hat{\mathbf{S}}_1 \cdot \hat{\mathbf{S}}_2 [\hat{P}_A \hat{P}_B + \hat{P}_B \hat{P}_A] \left| m^{\uparrow} n^{\uparrow} \right\rangle\,, \tag{5}
$$

which using Eq. 4 becomes

$$
\begin{aligned}
A \;=\; \sum_{m,n} \Bigg[ & \left\langle m^{\uparrow} n^{\uparrow} \right| \hat{S}_z(1)\hat{S}_z(2)[\hat{P}_A \hat{P}_B + \hat{P}_B \hat{P}_A] \left| m^{\uparrow} n^{\uparrow} \right\rangle \\
& + \frac{1}{2}[\left\langle m^{\uparrow} n^{\uparrow} \right| [\hat{S}^+(1)\hat{S}^-(2)[\hat{P}_A \hat{P}_B + \hat{P}_B \hat{P}_A] \left| m^{\uparrow} n^{\uparrow} \right\rangle \\
& + \left\langle m^{\uparrow} n^{\uparrow} \right| \hat{S}^-(1)\hat{S}^+(2)][\hat{P}_A \hat{P}_B + \hat{P}_B \hat{P}_A] \left| m^{\uparrow} n^{\uparrow} \right\rangle] \Bigg] .
\end{aligned} \tag{6}
$$

Simplifying, this gives

$$
A = \frac{1}{4} \sum_{m,n} \left\langle m^{\uparrow} n^{\uparrow} \right| [\hat{P}_A \hat{P}_B + \hat{P}_B \hat{P}_A] \left| m^{\uparrow} n^{\uparrow} \right\rangle + 0 + 0\,.
$$

or

$$A = \frac{1}{2}\sum_{m,n} \left\langle m^{\uparrow} \middle| \hat{P}_A \middle| m^{\uparrow} \right\rangle \left\langle n^{\uparrow} \middle| \hat{P}_B \middle| n^{\uparrow} \right\rangle \tag{7}$$

Similarly, the $B$, $C$, and $E$ terms are:

$$B = \frac{1}{2}\sum_{m,n} \left\langle m^{\uparrow} \middle| \hat{P}_A \middle| n^{\uparrow} \right\rangle \left\langle n^{\uparrow} \middle| \hat{P}_B \middle| m^{\uparrow} \right\rangle$$
$$C = \frac{1}{2}\sum_{m,n} \left\langle m^{\downarrow} \middle| \hat{P}_A \middle| m^{\downarrow} \right\rangle \left\langle n^{\downarrow} \middle| \hat{P}_B \middle| n^{\downarrow} \right\rangle$$
$$D = \frac{1}{2}\sum_{m,n} \left\langle m^{\downarrow} \middle| \hat{P}_A \middle| n^{\downarrow} \right\rangle \left\langle n^{\downarrow} \middle| \hat{P}_B \middle| m^{\downarrow} \right\rangle$$

The mixed-spin terms ($E$-$H$) can also be reduced using Eq. 4:

$$\begin{aligned} E \quad = \quad & \sum_{m,n} \Big[ \left\langle m^{\uparrow} n^{\downarrow} \middle| \hat{S}_z(1)\hat{S}_z(2)[\hat{P}_A\hat{P}_B + \hat{P}_B\hat{P}_A] \middle| m^{\uparrow} n^{\downarrow} \right\rangle \\ & + \frac{1}{2}[\left\langle m^{\uparrow} n^{\downarrow} \middle| [\hat{S}^{+}(1)\hat{S}^{-}(2)[\hat{P}_A\hat{P}_B + \hat{P}_B\hat{P}_A] \middle| m^{\uparrow} n^{\downarrow} \right\rangle \\ & + \left\langle m^{\uparrow} n^{\downarrow} \middle| \hat{S}^{-}(1)\hat{S}^{+}(2)][\hat{P}_A\hat{P}_B + \hat{P}_B\hat{P}_A] \middle| m^{\uparrow} n^{\downarrow} \right\rangle] \Big] \end{aligned}$$

or

$$E = \sum_{m,n} \left[ -\frac{1}{4} \left\langle m^{\uparrow} n^{\downarrow} \middle| [\hat{P}_A\hat{P}_B + \hat{P}_B\hat{P}_A] \middle| m^{\uparrow} n^{\downarrow} \right\rangle + 0 + \frac{1}{2}\sum_{m,n} \left\langle m^{\uparrow} n^{\downarrow} \middle| [\hat{P}_A\hat{P}_B + \hat{P}_B\hat{P}_A] \middle| m^{\downarrow} n^{\uparrow} \right\rangle \right]$$

$$= \sum_{m,n} \left[ -\frac{1}{2} \left\langle m^{\uparrow} \middle| \hat{P}_A \middle| m^{\uparrow} \right\rangle \left\langle n^{\downarrow} \middle| \hat{P}_B \middle| n^{\downarrow} \right\rangle + 0 + \sum_{m,n} \left\langle m^{\uparrow} \middle| \hat{P}_A \middle| m^{\downarrow} \right\rangle \left\langle n^{\downarrow} \middle| \hat{P}_B \middle| n^{\uparrow} \right\rangle \right]. \tag{8}$$

Similarly, the terms $F$-$H$ can be expressed as:

$$
\begin{aligned}
F &= \sum_{m,n}\Bigg[\left\langle m^{\uparrow}n^{\downarrow}\middle|\hat{S}_z(1)\hat{S}_z(2)[\hat{P}_A\hat{P}_B+\hat{P}_B\hat{P}_A]\middle|n^{\downarrow}m^{\uparrow}\right\rangle \\
&\quad +\frac{1}{2}[\left\langle m^{\uparrow}n^{\downarrow}\middle|[\hat{S}^{+}(1)\hat{S}^{-}(2)[\hat{P}_A\hat{P}_B+\hat{P}_B\hat{P}_A]\middle|n^{\downarrow}m^{\uparrow}\right\rangle \\
&\quad +\left\langle m^{\uparrow}n^{\downarrow}\middle|\hat{S}^{-}(1)\hat{S}^{+}(2)[\hat{P}_A\hat{P}_B+\hat{P}_B\hat{P}_A]\middle|n^{\downarrow}m^{\uparrow}\right\rangle]\Bigg] \\
&= \sum_{m,n}\Bigg[-\frac{1}{2}\left\langle m^{\uparrow}\middle|\hat{P}_A\middle|n^{\downarrow}\right\rangle\left\langle n^{\downarrow}\middle|\hat{P}_B\middle|m^{\uparrow}\right\rangle \\
&\quad +\left\langle m^{\uparrow}\middle|\hat{P}_A\middle|n^{\uparrow}\right\rangle\left\langle n^{\downarrow}\middle|\hat{P}_B\middle|m^{\downarrow}\right\rangle+0\Bigg], \qquad (9)
\end{aligned}
$$

$$
\begin{aligned}
G &= \sum_{m,n}\Bigg[\left\langle m^{\downarrow}n^{\uparrow}\middle|\hat{S}_z(1)\hat{S}_z(2)[\hat{P}_A\hat{P}_B+\hat{P}_B\hat{P}_A]\middle|m^{\downarrow}n^{\uparrow}\right\rangle \\
&\quad +\frac{1}{2}[\left\langle m^{\downarrow}n^{\uparrow}\middle|[\hat{S}^{+}(1)\hat{S}^{-}(2)[\hat{P}_A\hat{P}_B+\hat{P}_B\hat{P}_A]\middle|m^{\downarrow}n^{\uparrow}\right\rangle \\
&\quad +\left\langle m^{\downarrow}n^{\uparrow}\middle|\hat{S}^{-}(1)\hat{S}^{+}(2)[\hat{P}_A\hat{P}_B+\hat{P}_B\hat{P}_A]\middle|m^{\downarrow}n^{\uparrow}\right\rangle]\Bigg] \\
&= \sum_{m,n}\Bigg[-\frac{1}{2}\left\langle m^{\downarrow}\middle|\hat{P}_A\middle|m^{\downarrow}\right\rangle\left\langle n^{\uparrow}\middle|\hat{P}_B\middle|n^{\uparrow}\right\rangle+0 \\
&\quad +\left\langle m^{\downarrow}\middle|\hat{P}_A\middle|m^{\uparrow}\right\rangle\left\langle n^{\uparrow}\middle|\hat{P}_B\middle|n^{\downarrow}\right\rangle\Bigg], \qquad (10)
\end{aligned}
$$

and

$$
\begin{aligned}
H &= \sum_{m,n}\Big[\left\langle m^{\downarrow}n^{\uparrow}\right|\hat{S}_z(1)\hat{S}_z(2)[\hat{P}_A\hat{P}_B+\hat{P}_B\hat{P}_A]\left|n^{\uparrow}m^{\downarrow}\right\rangle \\
&\quad +\frac{1}{2}[\left\langle m^{\downarrow}n^{\uparrow}\right|[\hat{S}^{+}(1)\hat{S}^{-}(2)[\hat{P}_A\hat{P}_B+\hat{P}_B\hat{P}_A]\left|n^{\uparrow}m^{\downarrow}\right\rangle \\
&\quad +\left\langle m^{\downarrow}n^{\uparrow}\right|\hat{S}^{-}(1)\hat{S}^{+}(2)[\hat{P}_A\hat{P}_B+\hat{P}_B\hat{P}_A]\left|n^{\uparrow}m^{\downarrow}\right\rangle\Big] \\
&= \sum_{m,n}\Big[-\frac{1}{2}\left\langle m^{\downarrow}\right|\hat{P}_A\left|n^{\uparrow}\right\rangle\left\langle n^{\uparrow}\right|\hat{P}_B\left|m^{\downarrow}\right\rangle+0 \\
&\quad +\left\langle m^{\downarrow}\right|\hat{P}_A\left|n^{\downarrow}\right\rangle\left\langle n^{\uparrow}\right|\hat{P}_B\left|m^{\uparrow}\right\rangle\Big]. \qquad (11)
\end{aligned}
$$

Substituting $A$ through $H$ in Eq. 3, we obtain Eq. 9 from the manuscript:

$$
\begin{aligned}
\left\langle \hat{\mathbf{S}}_A\cdot\hat{\mathbf{S}}_B\right\rangle &= \frac{3}{4}\delta_{AB}\sum_{m}\left[\left\langle m^{\uparrow}\right|\hat{P}_A\left|m^{\uparrow}\right\rangle+\left\langle m^{\downarrow}\right|\hat{P}_A\left|m^{\downarrow}\right\rangle\right]+ \\
&\quad \sum_{m,n}\Big[\frac{1}{4}\left\langle m^{\uparrow}\right|\hat{P}_A\left|m^{\uparrow}\right\rangle\left\langle n^{\uparrow}\right|\hat{P}_B\left|n^{\uparrow}\right\rangle+\frac{1}{4}\left\langle m^{\downarrow}\right|\hat{P}_A\left|m^{\downarrow}\right\rangle\left\langle n^{\downarrow}\right|\hat{P}_B\left|n^{\downarrow}\right\rangle \\
&\quad -\frac{1}{4}\left\langle m^{\uparrow}\right|\hat{P}_A\left|n^{\uparrow}\right\rangle\left\langle n^{\uparrow}\right|\hat{P}_B\left|m^{\uparrow}\right\rangle-\frac{1}{4}\left\langle m^{\downarrow}\right|\hat{P}_A\left|n^{\downarrow}\right\rangle\left\langle n^{\downarrow}\right|\hat{P}_B\left|m^{\downarrow}\right\rangle \\
&\quad -\frac{1}{4}\left\langle m^{\uparrow}\right|\hat{P}_A\left|m^{\uparrow}\right\rangle\left\langle n^{\downarrow}\right|\hat{P}_B\left|n^{\downarrow}\right\rangle-\frac{1}{4}\left\langle m^{\downarrow}\right|\hat{P}_A\left|m^{\downarrow}\right\rangle\left\langle n^{\uparrow}\right|\hat{P}_B\left|n^{\uparrow}\right\rangle \\
&\quad -\frac{1}{2}\left\langle m^{\uparrow}\right|\hat{P}_A\left|n^{\uparrow}\right\rangle\left\langle n^{\downarrow}\right|\hat{P}_B\left|m^{\downarrow}\right\rangle-\frac{1}{2}\left\langle m^{\downarrow}\right|\hat{P}_A\left|n^{\downarrow}\right\rangle\left\langle n^{\uparrow}\right|\hat{P}_B\left|m^{\uparrow}\right\rangle \\
&\quad +\frac{1}{2}\left\langle m^{\uparrow}\right|\hat{P}_A\left|m^{\downarrow}\right\rangle\left\langle n^{\downarrow}\right|\hat{P}_B\left|n^{\uparrow}\right\rangle+\frac{1}{2}\left\langle m^{\downarrow}\right|\hat{P}_A\left|m^{\uparrow}\right\rangle\left\langle n^{\uparrow}\right|\hat{P}_B\left|n^{\downarrow}\right\rangle \\
&\quad +\frac{1}{4}\left\langle m^{\uparrow}\right|\hat{P}_A\left|n^{\downarrow}\right\rangle\left\langle n^{\downarrow}\right|\hat{P}_B\left|m^{\uparrow}\right\rangle+\frac{1}{4}\left\langle m^{\downarrow}\right|\hat{P}_A\left|n^{\uparrow}\right\rangle\left\langle n^{\uparrow}\right|\hat{P}_B\left|m^{\downarrow}\right\rangle.\Big], \qquad (12)
\end{aligned}
$$

which can be expressed in terms of projected one-particle density matrices as:

$$
\begin{aligned}
\left\langle \hat{\mathbf{S}}_A \cdot \hat{\mathbf{S}}_B \right\rangle &= \frac{3}{4}\delta_{AB}\sum_{\mu\in A}\left[\mathbf{P}^{\uparrow\uparrow}_{\mu\mu}+\mathbf{P}^{\downarrow\downarrow}_{\mu\mu}\right]+\sum_{\mu\in A,\nu\in B}\left[\frac{1}{4}\mathbf{P}^{\uparrow\uparrow}_{\mu\mu}\mathbf{P}^{\uparrow\uparrow}_{\nu\nu}+\frac{1}{4}\mathbf{P}^{\downarrow\downarrow}_{\mu\mu}\mathbf{P}^{\downarrow\downarrow}_{\nu\nu}\right.\\
&-\frac{1}{4}\mathbf{P}^{\uparrow\uparrow}_{\mu\nu}\mathbf{P}^{\uparrow\uparrow}_{\nu\mu}-\frac{1}{4}\mathbf{P}^{\downarrow\downarrow}_{\mu\nu}\mathbf{P}^{\downarrow\downarrow}_{\nu\mu}-\frac{1}{4}\mathbf{P}^{\uparrow\uparrow}_{\mu\mu}\mathbf{P}^{\downarrow\downarrow}_{\nu\nu}-\frac{1}{4}\mathbf{P}^{\downarrow\downarrow}_{\mu\mu}\mathbf{P}^{\uparrow\uparrow}_{\nu\nu}-\frac{1}{2}\mathbf{P}^{\uparrow\uparrow}_{\mu\nu}\mathbf{P}^{\downarrow\downarrow}_{\nu\mu}\\
&\left.-\frac{1}{2}\mathbf{P}^{\downarrow\downarrow}_{\mu\nu}\mathbf{P}^{\uparrow\uparrow}_{\nu\mu}+\frac{1}{2}\mathbf{P}^{\uparrow\downarrow}_{\mu\mu}\mathbf{P}^{\downarrow\uparrow}_{\nu\nu}+\frac{1}{2}\mathbf{P}^{\downarrow\uparrow}_{\mu\mu}\mathbf{P}^{\uparrow\downarrow}_{\nu\nu}+\frac{1}{4}\mathbf{P}^{\uparrow\downarrow}_{\mu\nu}\mathbf{P}^{\downarrow\uparrow}_{\nu\mu}+\frac{1}{4}\mathbf{P}^{\downarrow\uparrow}_{\mu\nu}\mathbf{P}^{\uparrow\downarrow}_{\nu\mu}\right]. \qquad (13)
\end{aligned}
$$

A more compact form of Eq. 13 can be derived by defining a vector $\vec{\mathbf{P}}_{\mu\nu}$ with cartesian components $\mathbf{P}^x_{\mu\nu}=\mathbf{P}^{\uparrow\downarrow}_{\mu\nu}+\mathbf{P}^{\uparrow\downarrow}_{\mu\nu}$, $\mathbf{P}^y_{\mu\nu}=i(\mathbf{P}^{\uparrow\downarrow}_{\mu\nu}-\mathbf{P}^{\uparrow\downarrow}_{\mu\nu})$, $\mathbf{P}^z_{\mu\nu}=\mathbf{P}^{\uparrow\uparrow}_{\mu\nu}-\mathbf{P}^{\downarrow\downarrow}_{\mu\nu}$, and scalor $\mathbf{P}_{\mu\nu}=\mathbf{P}^{\uparrow\uparrow}_{\mu\nu}+\mathbf{P}^{\downarrow\downarrow}_{\mu\nu}$. From these relations, we can write,

$$
\begin{aligned}
\mathbf{P}^{\uparrow\downarrow}_{\mu\nu} &= \frac{1}{2}(\mathbf{P}^x_{\mu\nu}-i\mathbf{P}^y_{\mu\nu})\\
\mathbf{P}^{\downarrow\uparrow}_{\mu\nu} &= \frac{1}{2}(\mathbf{P}^x_{\mu\nu}+i\mathbf{P}^y_{\mu\nu})\\
\mathbf{P}^{\uparrow\uparrow}_{\mu\nu} &= \frac{1}{2}(\mathbf{P}_{\mu\nu}+\mathbf{P}^z_{\mu\nu})\\
\mathbf{P}^{\downarrow\downarrow}_{\mu\nu} &= \frac{1}{2}(\mathbf{P}_{\mu\nu}-\mathbf{P}^z_{\mu\nu})
\end{aligned}
$$

Substituting these in Eq. 13 and working the algebra algebra, one obtains:

$$
\begin{aligned}
\left\langle \hat{\mathbf{S}}_A \cdot \hat{\mathbf{S}}_B \right\rangle &= \frac{3}{4}\delta_{AB}\mathbf{P}_{\mu\mu}+\frac{1}{4}[\frac{1}{2}(\mathbf{P}^z_{\mu\mu}\mathbf{P}^z_{\nu\nu}+\mathbf{P}_{\mu\mu}\mathbf{P}_{\nu\nu})]-\frac{1}{4}[\frac{1}{2}(\mathbf{P}^z_{\mu\nu}\mathbf{P}^z_{\nu\mu}+\mathbf{P}_{\mu\nu}\mathbf{P}_{\nu\mu})]\\
&-\frac{1}{4}[\frac{1}{2}(-\mathbf{P}^z_{\mu\mu}\mathbf{P}^z_{\nu\nu}+\mathbf{P}_{\mu\mu}\mathbf{P}_{\nu\nu})]-\frac{1}{2}[\frac{1}{2}(-\mathbf{P}^z_{\mu\nu}\mathbf{P}^z_{\nu\mu}+\mathbf{P}_{\mu\nu}\mathbf{P}_{\nu\mu})]+\\
&\frac{1}{2}[\frac{1}{2}(\mathbf{P}^x_{\mu\mu}\mathbf{P}^x_{\nu\nu}+\mathbf{P}^y_{\mu\mu}\mathbf{P}^y_{\nu\nu})]+\frac{1}{4}[\frac{1}{2}\ (\mathbf{P}^x_{\mu\nu}\mathbf{P}^x_{\nu\mu}+\mathbf{P}^y_{\mu\nu}\mathbf{P}^y_{\nu\mu})], \qquad (14)
\end{aligned}
$$

where we have dropped the summations for simplicity. Combining terms we have

$$\langle \hat{\mathbf{S}}_A \cdot \hat{\mathbf{S}}_B \rangle = \frac{3}{4}\delta_{AB}\mathbf{P}_{\mu\mu} + \frac{1}{4}[\mathbf{P}^x_{\mu\mu}\mathbf{P}^x_{\nu\nu} + \mathbf{P}^y_{\mu\mu}\mathbf{P}^y_{\nu\nu} + \mathbf{P}^z_{\mu\mu}\mathbf{P}^z_{\nu\nu}]$$
$$+\frac{1}{8}[\mathbf{P}^x_{\mu\nu}\mathbf{P}^x_{\nu\mu} + \mathbf{P}^y_{\mu\nu}\mathbf{P}^y_{\nu\mu} + \mathbf{P}^z_{\mu\nu}\mathbf{P}^z_{\nu\mu}] - \frac{3}{8}\mathbf{P}_{\mu\nu}\mathbf{P}_{\mu\nu} \tag{15}$$

and rewritting this expression as

$$\langle \hat{\mathbf{S}}_A \cdot \hat{\mathbf{S}}_B \rangle = \frac{3}{4}(\delta_{AB}\mathbf{P}_{\mu\mu} - \frac{1}{2}\mathbf{P}_{\mu\nu}\mathbf{P}_{\nu\mu}) + \frac{1}{4}(\vec{\mathbf{P}}_{\mu\mu} \cdot \vec{\mathbf{P}}_{\nu\nu} + \frac{1}{2}\vec{\mathbf{P}}_{\mu\nu} \cdot \vec{\mathbf{P}}_{\nu\mu}). \tag{16}$$

Replacing the notation $\sum_{\mu\in A}$ and $\sum_{\nu\in B}$ with subindices $A$ and $B$, we obtain Eq. 11 of the main text:

$$\langle \hat{\mathbf{S}}_A \cdot \hat{\mathbf{S}}_B \rangle = \frac{3}{4}(\delta_{AB}\mathbf{P}_{AA} - \frac{1}{2}\mathbf{P}_{AB}\mathbf{P}_{BA}) + \frac{1}{4}(\vec{\mathbf{P}}_{AA} \cdot \vec{\mathbf{P}}_{BB} + \frac{1}{2}\vec{\mathbf{P}}_{AB} \cdot \vec{\mathbf{P}}_{BA}). \tag{17}$$

## xyz Coordinates of the $[(Mn^4)_3O_4L_4(H_2O)]$ complex

Mn -1.337475 0.000000 0.000000

Mn 1.342218 0.000000 0.000000

Mn 0.000000 0.000000 -2.982529

O 0.034052 1.200611 0.192426

O -0.029047 -1.199108 0.200738

O -1.324097 0.032363 -1.806643

O 1.324148 -0.034859 -1.807201

O -2.850328 1.523388 -0.183803

H -3.562810 1.373748 -0.840551

H -3.287200 1.938333 0.590868

O 2.843692 -1.538262 -0.192931

H 3.570948 -1.380000 -0.831336

H 3.262879 -1.970666 0.582092

N -2.857627 -1.442896 0.179206

N -1.820394 0.129792 2.044717

C -3.270353 -1.640016 1.504506

H -4.011974 -2.409746 1.729511

C -2.749507 -0.838609 2.450485

H -3.039811 -0.902219 3.501678

C -3.384877 -2.130296 -0.774635

H -4.155178 -2.885147 -0.580671

H -3.057163 -1.942672 -1.796437

C -1.384282 1.019597 2.871403

H -1.725148 1.047152 3.913428

H -0.672919 1.764035 2.510134

N 2.871919 1.434365 0.168008

N 1.831267 -0.123939 2.043028

C 3.290812 1.634216 1.490941

H 4.038048 2.400166 1.710131

C 2.767952 0.840051 2.441857

H 3.061993 0.905955 3.491835

C 3.399868 2.114592 -0.790656

H 4.175370 2.865587 -0.602578

H 3.066737 1.925091 -1.810354

C 1.392914 -1.007609 2.875169

H 1.738621 -1.033620 3.915614

H 0.675144 -1.748772 2.519931

N 1.407049 0.151523 -4.581475

N 0.110045 2.036789 -3.199373

C 1.658844 1.495434 -4.895271

H 2.360270 1.737623 -5.697498

C 1.009147 2.443168 -4.199592

H 1.143177 3.510146 -4.391802

C 2.000949 -0.772153 -5.257841

H 2.698601 -0.528333 -6.067469

H 1.810909 -1.821410 -5.037435

C -0.520178 2.914752 -2.494848

H -0.367300 3.986422 -2.666658

H -1.207234 2.581040 -1.720601

N -1.413015 -0.150614 -4.576487

N -0.109851 -2.036405 -3.201246

C -1.666070 -1.494328 -4.889981

H -2.370980 -1.736097 -5.689272

C -1.013741 -2.442396 -4.197256

H -1.148613 -3.509296 -4.389319

C -2.010266 0.773481 -5.249237

H -2.714326 0.530267 -6.053490

H -1.819717 1.822585 -5.028464

C 0.525104 -2.914375 -2.501032

H 0.372591 -3.986000 -2.673493

H 1.216046 -2.580441 -1.730213

## xyz Coordinates of the $(\mu - OCH_3VO(ma)]_2$ complex

V 0.933423136 1.16726372 0.372422819

V -0.933423136 -1.16726372 -0.372422819

O -0.0700049576 -0.33042 1.15800644

O 0.0700049576 0.33042 -1.15800644

O 5.90071107 1.569495 1.28536908

O 2.39817005 0.787501 1.58345186

O 2.45641842 1.778761 -0.79940382

O 0.180746881 2.5089892 0.765079136

C 4.89661546 0.473602 3.14612825

C 4.7420872 1.1025014 1.82282137

C 3.57782962 1.2236554 1.12277847

C 3.58154222 1.7754568 -0.175236544

C 4.81022296 2.2600728 -0.694623206

C 5.89627869 2.1400202 0.053293588

C -0.032677831 -0.7500534 2.51834785

H 4.78159995 0.958218 3.71248554

H 4.12440793 -0.088112 3.40536994

H 5.61133587 -0.088112 3.2879434

H 4.89763819 2.577276 -1.56267639

H 6.79481052 2.390038 -0.171623419

H -0.704359343 -1.189512 2.78210595

H 0.214483688 0.022028 3.24277934

H 0.667447647 -1.343708 2.62854815

O -5.90071107 -1.569495 -1.28536908

O -2.39817005 -0.787501 -1.58345186

O -2.45641842 -1.778761 0.79940382

O -0.180746881 -2.5089892 -0.765079136

C -4.89661546 -0.473602 -3.14612825

C -4.7420872 -1.1025014 -1.82282137

C -3.57782962 -1.2236554 -1.12277847

C -3.58154222 -1.7754568 0.175236544

C -4.81022296 -2.2600728 0.694623206

C -5.89627869 -2.1400202 -0.053293588

C 0.032677831 0.7500534 -2.51834785

H -4.78159995 -0.958218 -3.71248554

H -4.12440793 0.088112 -3.40536994

H -5.61133587 0.088112 -3.2879434

H -4.89763819 -2.577276 1.56267639

H -6.79481052 -2.390038 0.171623419

H 0.704359343 1.189512 -2.78210595

H -0.214483688 -0.022028 -3.24277934

H -0.667447647 1.343708 -2.62854815

# References

**S1**. Luo, S.; I. Rivalta, V. B.; Truhlar, D. G. Noncollinear Spins Provide a Self-Consistent Treatment of the Low-Spin State of a Biomimetic Oxomanganese Synthetic Trimer Inspired by the Oxygen Evolving Complex of Photosystem II. *Phys. Chem. Lett.* **2012**, 2, 2629−2633.

**S2**. Sun, Y.; Melchior, M.; Summers, D. A.; Thompson, R. C.; Rettig, S. J.; Orvig, C. $[(\mu - OCH_3VO(ma)]_2$, A Strongly Antiferromagnetic Oxovanadium(IV) Dimer. *Inorg. Chem.* **1998**, 37, 3119.
